# Supplementary material for: Do Large Language Models Understand Performance Optimization?
Source: arXiv:2503.13772 source file (2025-03-17)
Supplement: Supplementary file 1 [file Appendix.tex]

\appendix
\label{appendix_optimization_list}
Table ~\ref{tab:Optimization-list} summarizes optimizations applied by Codee and LLMs in our experiments.\\
\noindent\textbf{List of Canonical Optimizations}
\begin{enumerate}
    \item Loop Nesting (LN): Rearranging loops to optimize for cache usage and performance.
    \item Loop Interchange (LI): Changing the order of nested loops to improve data locality.
    \item Loop Unrolling (LU): Expanding the loop to decrease the overhead of loop control.
    \item Loop Tiling (LT): Dividing loops into smaller blocks to enhance cache performance.
    \item Loop Fission (LF): Splitting a loop into multiple loops over the same index range.
    \item Loop Fusion (LFU): Combining multiple loops into a single loop to improve locality.
    \item Fused Multiply-Add (FMA): Combining multiply and add operations into a single instruction.
    \item Change of Precision (COP): Adjusting the precision of calculations to enhance performance.
    \item Attribute (pure) (ATT): Marking functions as pure for better optimization opportunities.
    \item Multithreading (MT): Using multiple threads to execute code segments concurrently.
    \item OpenMP Scoping (OS): Defining the scope of variables within OpenMP parallel regions.
    \item OpenMP Vectorization (OV): Applying vectorization techniques using OpenMP directives.
\end{enumerate}

\noindent\textbf{List of Additional LLM-Generated Optimizations}
\begin{enumerate}
    \item Memory Optimization (MO): Techniques to reduce memory usage and improve data access patterns.
    \item Cache Blocking (CB): Dividing data into blocks to fit in cache, reducing repeated access overhead.
    \item Pre-Computing Constants (PCC): Calculating constants before runtime to save computational overhead.
    \item Mathematical Simplification (MS): Simplifying mathematical expressions to reduce computation time.
    \item Reducing Function Overhead (RFO): Minimizing the overhead caused by frequent function calls.
    \item SIMD Optimizations (SI): Using Single Instruction Multiple Data (SIMD) to parallelize operations.
    \item OpenMP Reduction (OR): Optimizing reduction operations using OpenMP to improve performance.
\end{enumerate}

\begin{table}[H]
\centering
\caption{Optimization Summary}
\label{tab:Optimization-list}
\resizebox{\columnwidth}{!}{%
\begin{tabular}{l l l}
  \midrule
  Tool     & Example        & Optimization Applied  \\
  \midrule
  Codee    & MATMUL         & LI,FMA,MT                \\
  ChatGPT-4    & MATMUL         & LI,LU,CB,MS           \\
  Llama3.1 & MATMUL         & LI,LU,CB              \\
  Codee    & ATMUX          & LF,FMA,MT                \\
  ChatGPT-4    & ATMUX          & LFU,MO,PCC,RFO        \\
  Llama3.1 & ATMUX          & LU,MO,CB,MS           \\
  Codee    & PI             & MS,MT                    \\
  ChatGPT-4    & PI             & LU,PCC,COP,OR            \\
  Llama3.1 & PI             & LU,CB,COP,MS,OR          \\
  Codee    & CANNY          & FMA,COP,MS,ATT,MT        \\
  ChatGPT-4    & CANNY          & LU,MO,RFO,OR,OS           \\
  Llama3.1 & CANNY          & OR,OS                   \\
  Codee    & COULOMB        & FMA,MS,MT                \\
  ChatGPT-4    & COULOMB        & LU,PCC,MS             \\
  Llama3.1 & COULOMB        & LU,MO,CB,PCC,RFO      \\
  Codee    & HACCmk         & MT,FMA,MS                   \\
  ChatGPT-4    & HACCmk         & MT,OR,MO                      \\
  Llama3.1 & HACCmk         & OR,MT                     \\
  Codee    & NPB\_CG        & MT,LF,FMA                   \\
  ChatGPT-4    & NPB\_CG        & MT,OR                   \\
  Llama3.1 & NPB\_CG        & OR,RFO                    \\
  Codee    & Hotspot        & FMA,COP,OS,MT          \\
  ChatGPT-4    & Hotspot        & LU,MO,CB,PCC,MS       \\
  Llama3.1 & Hotspot        & LI,LU,MO,CB,RFO        \\
  Codee    & Hotspot3D      & MO,FMA,COP,MS,ATT,OS,OV \\
  ChatGPT-4    & Hotspot3D      & LI,LU,MO,COP,RFO      \\
  Llama3.1 & Hotspot3D      & LU,CB                 \\
  Codee    & Particlefilter & LF,MO,FMA,MS,ATT,OS,OV  \\
  ChatGPT-4    & Particlefilter & LI,LU,MO,RFO,OR      \\
  Codee    & Srad           & LF,FMA,COP,OS,OV       \\
  ChatGPT-4    & Srad           & LU,LT,MO,COP,OR      \\
  Llama3.1 & Srad           & LU,MO,RFO,OR        \\
  Codee    & Qsort          & MS,ATT                      \\
  ChatGPT-4    & Qsort          & MS,RFO,MO                    \\
  Llama3.1 & Qsort          & MS,RFO,LU,CB,SI                     \\
  Codee    & Sha            & OV,                     \\
  ChatGPT-4    & Sha            & LU,MO,RFO                      \\
  Llama3.1 & Sha            & LU,SI,MO                      \\
  Codee    & Susan          & OV,ATT,COP                     \\
  Codee    & FFT            & COP,FMA                      \\
  ChatGPT-4    & FFT            & MS,MO,LU,RFO                      \\
  Llama3.1 & FFT            & RFO,MO,LU,CB,SI                     \\
  \midrule
\end{tabular}
}
\end{table}

%\caption{Summary of Optimizations Applied\tablefootnote{LN = Loop Nesting, LR = Loop Reordering, LU = Loop Unrolling, LT = Loop Tiling, LF = Loop Fission, LFU = Loop Fusion, MO = Memory Optimization, CB = Cache Blocking, PCC = Pre-Computing Constants, FMA = Fused Multiply-Add, COP = Change of Precision, MS = Mathematical Simplification, RFO = Reducing Function Overhead, ATT = \_\_attribute\_\_(pure), MT=Multithreading OV = OpenMP Scoping, OV = OpenMP Vectorization, OR = OpenMP Reduction, SI=SIMD Optimizations.}}
